# Supplementary material for: DP-UTIL: Comprehensive Utility Analysis of Differential Privacy in Machine Learning
Source: arXiv:2112.12998 source file (2021-12-24)
Supplement: Supplementary file 1 [file appendix.tex]

\section{Appendix}\label{sec: Appendix}
